# Supplementary material for: Dynamic cluster structure and predictive modelling of music creation style distributions
Source: arXiv:2205.13923 ancillary file (2022-05-27)
Supplement: Supplementary file 1 [file Supple.pdf]

# Supplemental Material for

# Dynamic cluster structure and predictive modelling of music creation style distributions

Rajsuryan Singh and Eita Nakamura

## Contents

**1 Evolution of syncopated rhythms in J-pop data** **1**

**2 State-space evolutionary model (SSEM)** **1**

2.1 Model formulation . . . . . . . . . . . . . . . . . . . . . . . . . . . . . . . 2

2.2 Prediction method . . . . . . . . . . . . . . . . . . . . . . . . . . . . . . . 3

**3 Melody generation using model predictions** **5**

**4 Data and code availability** **5**

## 1 Evolution of syncopated rhythms in J-pop data

In Fig. 2 in the main text, we observed the shift of the centre of cluster 4 in rhythm statistics extracted from the J-pop dataset. Here, we show that this shift represents the movement towards widely utilizing syncopated rhythms. To examine this, we defined syncopated rhythms as rhythms involving musical notes extending across strong beat positions. Specifically, we defined the probability of syncopated rhythms as the sum of the bigram probabilities of metrical positions $(b', b)$ that satisfy $b' < 24 < b$ or $0 < b < b'$ (0 and 24 represent the downbeat and the middle of a bar, respectively).

Fig. 1(c) illustrates the probability of syncopated rhythms for individual songs, where the colour depends on the square root of the probability. In the region corresponding to cluster 4, the probability values correlate with the vertical positions, demonstrating that the shift of the cluster occuring between the 1960s and the 1980s represents a transition to utilizing more frequent syncopated rhythms.

## 2 State-space evolutionary model (SSEM)

In Sec. 3.3 in the main text, we described the state-space evolutionary model (SSEM). We here formulate the model more systematically and present the algorithms for fitness estimation and prediction.

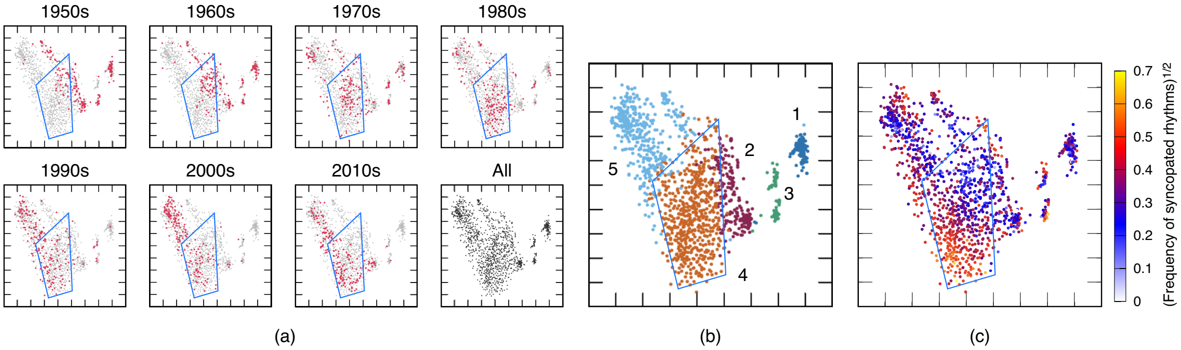


Figure 1: The evolutions of the distribution and cluster structure of the rhythm statistics in the J-pop data. (a) The two-dimensional visualization of the data distribution. (b) Result of the cluster analysis with $K = 5$. (c) Probability of syncopated rhythms. Panels (a) and (b) are reproduced from Fig. 2 in the main article.

### 2.1 Model formulation

As explained in Sec. 3.3 in the main text, the SSEM for a variable $x(t)$ with the velocity (logarithm of the normalized fitness) and acceleration variables $v(t)$ and $a(t)$, respectively, is defined as

$$x(t+1) = x(t) + v(t) + \epsilon(t), \tag{1}$$

$$v(t+1) = v(t) + \eta(t), \tag{2}$$

where $\epsilon(t)$ and $\eta(t)$ are Gaussian noises. To formulate the model in the standard form of the state-space model [1] and extend it to including an arbitrary order of time derivatives, we introduce latent variables $\boldsymbol{z}(t) = [z_0(t)\ z_1(t)\ z_2(t)\ \cdots\ z_L(t)]^{\mathrm{T}}$, where $z_1(t) = v(t)$, and $z_2(t)$ etc. represent possible higher-order time derivatives; $L$ is the order of the model and we adopt a model with $L = 1$ in the analysis. The variable $z_0(t)$ is interpreted as the position variable $x(t)$ without noise (see Eq. (4) below). The state-space model is then formulated as

$$\boldsymbol{z}(t+1) = A\boldsymbol{z}(t) + \boldsymbol{\eta}(t), \quad A_{ij} = \begin{cases} 1 & (j = i, i+1); \\ 0 & \text{otherwise}, \end{cases} \tag{3}$$

$$x(t) = z_0(t) + \epsilon(t) = C\boldsymbol{z}(t) + \epsilon(t), \quad C = \begin{bmatrix} 1 & 0 & \cdots & 0 \end{bmatrix}. \tag{4}$$

The noise variables $\boldsymbol{\eta}(t) = [\eta_0(t)\ \eta_1(t)\ \cdots\ \eta_L(t)]^{\mathrm{T}}$ follow Gaussian distributions: $\langle \eta_l(t) \rangle = 0$ and $\langle \eta_l(t)\eta_{l'}(s) \rangle = \lambda_l^2 \delta_{ll'} \delta_{ts}$. Variable $\eta_1(t)$ corresponds to variable $\eta(t)$ in Eq. (2). Similarly, $\langle \epsilon(t) \rangle = 0$ and $\langle \epsilon(t)\epsilon(s) \rangle = \sigma^2 \delta_{ts}$. Standard deviation $\sigma$ represents the amount of observation noise, and standard deviation $\lambda_l$ represents the amount of time variations of $z_l$. We assume that $\lambda_0 = 0$ and treat $z_0(t)$ as an auxiliary variable.

To complete the model, we need to describe how the initial latent variables $z_l(1)$ are determined. We also treat them as stochastic variables following Gaussian distributions.

Together with Eqs. (3) and (4), the complete model is described as follows:

$$P(\boldsymbol{z}(1)) = N(\boldsymbol{z}(1); \boldsymbol{z}_{\rm ini}, \Lambda), \tag{5}$$

$$P(\boldsymbol{z}(t+1)|\boldsymbol{z}(t)) = N(\boldsymbol{z}(t+1); A\boldsymbol{z}(t), \Lambda) \quad (t = 2, 3, \ldots), \tag{6}$$

$$P(x(t)|\boldsymbol{z}(t)) = N(x(t); C\boldsymbol{z}(t), \Sigma) \quad (t = 1, 2, \ldots), \tag{7}$$

where $N(\,\cdot\,; \boldsymbol{\mu}, \Xi)$ denotes a Gaussian distribution with mean vector $\boldsymbol{\mu}$ and covariance matrix $\Xi$, $\Lambda = \mathrm{diag}[\lambda_0^2, \lambda_1^2, \ldots, \lambda_L^2]$, and $\Sigma = \sigma^2$. In addition to the variables $z_l(t)$ and $x(t)$, the model has parameters $z_{\mathrm{ini},l}$, $\lambda_l$, and $\sigma$, which should be fixed to make predictions. How to fix these values is explained below.

## 2.2 Prediction method

The prediction problem using the SSEM can be formalized as follows. Given a sequence of past data $x(1), \ldots, x(t_0)$ up to the referential time $t_0$, we use the model to predict the future values $x(t_0+1), x(t_0+2)$, etc. We should remark that here the time index has only a relative meaning. For example, since we only have a finite samples of past data, we can index the time for the first sample with $t = 1$, and then $t_0$ denotes the referential time counted from this first sample. In our analysis, we use a limited set of past data because the analysis in Section 2 in the main text revealed that the cluster structure of music styles change drastically in 10 to 20 years. More specifically, we use all the available past data after time $t_0 - 20$ (yrs). We index the time of the first sample in this selected data with $t = 1$ and redefined $t_0$ to indicate the referential year counted from this sample.

To apply the SSEM for predicting future values, we use the Kalman filter and Kalman smoothing algorithms, which are equivalent to the forward and backward algorithms for hidden Markov models, respectively [1]. By applying these algorithms we can compute the mean vector $\hat{\boldsymbol{z}}(t)$ and covariance matrix $\hat{\Lambda}$ of the posterior probability $P(\boldsymbol{z}(t)|x(1), \ldots, x(t_0))$ for $t = 1, \ldots, t_0$. This is a well-known result in statistics and readers should refer to [1] for explicit algorithms for computation.

The steps for making predictions are as follows. First, we fix the model parameters $z_{\mathrm{ini},l}$, $\lambda_l$, and $\sigma$ as follows. We initialize these values as $z_{\mathrm{ini},0} = x(1)$, $z_{\mathrm{ini},l} = 0$ $(l \geq 1)$, $\lambda_0 = 0$, $\lambda_l = \sigma_v$ $(l \geq 1)$, and $\sigma = \sigma_{\mathrm{data}}$, where $\sigma_v$ is a hyperparameter to be optimized and $\sigma_{\mathrm{data}}$ is the standard deviations of samples $\{x(1), \ldots, x(t_0)\}$. We then use the expectation-maximization (EM) algorithm to automatically optimize the initial values $\boldsymbol{z}_{\rm ini}$ by the maximum likelihood method. Specifically, in each iteration, we apply the forward and backward algorithms and update the values as $z_{\mathrm{ini},l} = \hat{z}_l(t = 1)$. The number of iterations was 10 in the analysis.

Next, we apply the forward-backward algorithm to estimate the latent variables $\hat{z}_l(t_0)$ at the referential time $t_0$. In particular, $\hat{z}_1(t_0)$ is interpreted as the estimated velocity (log fitness) at time $t_0$. The predictions for the future data are derived by maximizing the probabilities $P(x(t)|x(1), \ldots, x(t_0))$. The result is given as

$$\hat{x}(t) = \hat{z}_0(t_0) + \hat{z}_1(t_0)(t - t_0) \tag{8}$$

with possible higher-order terms in the general case with $L \geq 2$. These predictions are optimal when the model completely describes the data. In reality, however, there are nonlinear

Table 1: Optimized values of parameters $\sigma_v$ and $r$. The pitch and rhythm statistics are for the J-pop dataset and the timbre and harmony statistics are for the US-pop dataset.

| Data | Parameter | $\sigma_v$ | $r$ |
|---|---|---|---|
| Pitch ($K = 5$) | Mixture probabilities | 0.078476 | 0.615848 |
| | Concentrations | 0.001 | 0.615848 |
| | Mean distributions | 0.00335982 | 0.112884 |
| Pitch ($K = 10$) | Mixture probabilities | 0.0379269 | 0.483293 |
| | Concentrations | 0.00695193 | 0.297635 |
| | Mean distributions | 0.001 | 0.01 |
| Rhythm ($K = 5$) | Mixture probabilities | 0.0483293 | 0.379269 |
| | Concentrations | 0.00335982 | 0.183298 |
| | Mean distributions | 0.001 | 0.01 |
| Rhythm ($K = 10$) | Mixture probabilities | 0.0615848 | 0.233572 |
| | Concentrations | 0.00263665 | 0.297635 |
| | Mean distributions | 0.001 | 0.01 |
| Timbre ($K = 5$) | Mixture probabilities | 0.001 | 1.0 |
| | Concentrations | 0.00127427 | 0.0545559 |
| | Mean distributions | 0.001 | 0.01 |
| Timbre ($K = 10$) | Mixture probabilities | 0.00263665 | 0.0695193 |
| | Concentrations | 0.001 | 0.01 |
| | Mean distributions | 0.001 | 0.01 |
| Harmony ($K = 5$) | Mixture probabilities | 0.1 | 0.379269 |
| | Concentrations | 0.0112884 | 0.143845 |
| | Mean distributions | 0.001 | 0.483293 |
| Harmony ($K = 10$) | Mixture probabilities | 0.1 | 0.379269 |
| | Concentrations | 0.00885867 | 0.01 |
| | Mean distributions | 0.0233572 | 0.0885867 |

effects in the data and the predictions based on the linear dynamics can become inaccurate in the long term. By a preliminary experiment, we found that the following form of predictions are often more accurate.

$$\hat{x}(t) = x(t_0) + r\hat{z}_1(t_0)(t - t_0).$$

Here, the coefficient $r < 1$ (called *fitness reduction factor*) reduces the effect of the fitness for the prediction and thus yields more "conservative" predictions. By using the observed value $x(t_0)$ instead of the smoothed value $\hat{z}_0(t_0)$, we can also reduce the risk that the model oversmoothes the data.

We optimize the values of $\sigma_v$ and $r$ for minimizing the prediction errors. We conducted a grid search in the intervals $[0.001, 0.1]$ (20 steps) for $\sigma_v$ and $[0.01, 1]$ (20 steps) for $r$. Table 1 shows the optimized values found for each set of analysis.

## 3 Melody generation using model predictions

The audio samples `melo_2019.mp3` and `melo_2040.mp3` in the accompanying data are generated using the pitch and rhythm statistics observed in 2019 and predicted in 2040 for the J-pop dataset. To generate the melody samples, we used the mean distributions of the fifth cluster of the pitch bigram statistics in Fig. 6 in the main text, convert the statistics to the transition probabilities of extended pitch classes, and generate the pitches by the random walk sampling. We used the mean distributions of the fifth cluster of the rhythm statistics in a similar manner, and use the generated metrical positions for the onset times of the melody notes.

## 4 Data and code availability

The music statistics data and source code used for the analysis, the data obtained by the analysis, and melody audio samples are available at
https://drive.google.com/drive/folders/1n0nu89NmseIBIENMTFcB7PUq080MvkFb?usp=sharing .

## References

[1] C. M. Bishop, *Pattern Recognition and Machine Learning*, Springer, 2006.
